# Supplementary material for: Rotons in Optical Excitation Spectra of Monolayer Semiconductors
Source: arXiv:1812.10494 ancillary file (2018-12-26)
Supplement: Supplementary file 1 [file supplemental.pdf]

# Supplemental Material: Rotons in the Optical Excitation Spectrum of Monolayer Semiconductors

Ovidiu Cotlet,[1,*] Dominik S. Wild,[2,†] Mikhail D. Lukin,[2] and Atac Imamoglu[1]

[1] *Institute of Quantum Electronics, ETH Zürich, CH-8093, Zürich, Switzerland*

[2] *Department of Physics, Harvard University, Cambridge, Massachusetts 02138, USA*

## COMPUTATIONAL DETAILS

To compute the exciton energy, we use the dielectrically screened Coulomb interaction described in the main text with $r_0 = 5.17\,\text{nm}$ [S1]. The Schrdinger equation is diagonalized numerically in a basis of angular momentum eigenstates of the electron. We include angular momentum quantum numbers up to $m = 5$ and employ a nonuniform grid (quadratically increasing spacing) of 1000 radial momenta from 0 to $0.5\,\text{Å}^{-1}$. The electron and hole masses used for the calculation are $m_e = 0.56m_0$, $m_h = 0.59m_0$, where $m_0$ [S2] denotes the mass of a free electron. All numerical integrations were performed using a trapezoidal rule, adjusting the grid size to reach convergence.

## OPTICAL DECAY RATES

To compute the emission spectrum and radiative decay rates, we start from the fully quantized light-matter interaction Hamiltonian [S3]

$$H_\gamma = \sum_{\mathbf{p},\mathbf{p}_z,\mathbf{q},\lambda} \boldsymbol{\mu} \cdot \hat{\mathbf{e}}_{\mathbf{p}+\mathbf{p}_z,\lambda} \sqrt{\frac{\nu_{\mathbf{p}+\mathbf{p}_z}}{2\varepsilon_0}} \gamma^\dagger_{\mathbf{p}+\mathbf{p}_z,\lambda} e_\mathbf{q} h_{\mathbf{p}-\mathbf{q}} + \text{h.c.} \tag{S1}$$

Here, the momenta $\mathbf{p}$ and $\mathbf{q}$ are confined to the plane of the $MoSe_2$ monolayer ($xy$ plane), while $\mathbf{p}_z$ is perpendicular to it. The operator $\gamma^\dagger_{\mathbf{p},\lambda}$ creates a photon with total momentum $\mathbf{p}$ and polarization $\lambda$, where $\hat{\mathbf{e}}_{\mathbf{p},\lambda}$ denotes the associated polarization vector. We further introduced the transition dipole matrix element between the conduction and the valence band, $\boldsymbol{\mu}$ and the photon dispersion, $\nu_\mathbf{p} = c|\mathbf{p}|$. Since the valence band hole is assumed to be in the $K$ valley, electrons in the $K'$ do not participate in the decay process.

The spontaneous emission rate $\Gamma$ of some initial state $|i\rangle$ can be determined using Fermi's Golden Rule,

$$\Gamma = 2\pi \sum_f |\langle f|H_\gamma|i\rangle|^2 \delta(\omega_i - \omega_f), \tag{S2}$$

where the sum runs over all final states $|f\rangle$. By assuming that the photonic part of $|i\rangle$ is in the vacuum state, this may be written as

$$\Gamma = \frac{\pi}{\varepsilon_0} \sum_{\mathbf{p},\mathbf{p}_z,\lambda} |\boldsymbol{\mu} \cdot \hat{\mathbf{e}}_{\mathbf{p}+\mathbf{p}_z,\lambda}|^2 \nu_{\mathbf{p}+\mathbf{p}_z} \sum_f \left| \langle f| \sum_\mathbf{q} e_\mathbf{q} h_{\mathbf{p}-\mathbf{q}} |i\rangle \right|^2 \delta(\omega_i - \omega_f - \nu_{\mathbf{p}+\mathbf{p}_z}), \tag{S3}$$

where the states $|i\rangle$ and $|f\rangle$ as well as their corresponding energies $\omega_i$ and $\omega_f$ now only include electronic degrees of freedom. We make use of the identity

$$\sum_\lambda \hat{\mathbf{e}}_{\mathbf{p}\lambda} \hat{\mathbf{e}}_{\mathbf{p}\lambda} = I - \frac{1}{p^2}\mathbf{p}\mathbf{p} \tag{S4}$$

and employ the fact that $\boldsymbol{\mu}$ is in the $xy$ plane to obtain

$$\Gamma = \frac{\pi\mu^2}{\varepsilon_0} \sum_{\mathbf{p},\mathbf{p}_z,\lambda} \left(1 - \frac{|\hat{\boldsymbol{\mu}} \cdot \mathbf{p}|^2}{p^2 + p_z^2}\right) \nu_{\mathbf{p}+\mathbf{p}_z} \sum_f \left| \langle f| \sum_\mathbf{q} e_\mathbf{q} h_{\mathbf{p}-\mathbf{q}} |i\rangle \right|^2 \delta(\omega_i - \omega_f - \nu_{\mathbf{p}+\mathbf{p}_z}), \tag{S5}$$

where $\hat{\boldsymbol{\mu}} = \boldsymbol{\mu}/|\boldsymbol{\mu}|$. Next, we switch variables from ($\mathbf{p}$, $\mathbf{p}_z$) to ($\mathbf{p}$, $\nu$), where $\nu = \sqrt{p^2 + p_z^2}$ (having set $c = 1$). This is accomplished in the integrand Eq. (S3) by letting

$$\sum_{\mathbf{p},\mathbf{p}_z} \to \frac{1}{2\pi} \int_{-\infty}^{\infty} \mathrm{d}p_z \sum_\mathbf{p} \to \frac{1}{\pi} \int_0^\infty \mathrm{d}\nu \sum_{|\mathbf{p}|<\nu} \frac{\nu}{\sqrt{1 - p^2/\nu^2}}. \tag{S6}$$

Defining the spectral decay rate

$$\Gamma = \int_0^\infty \mathrm{d}\nu\, \Gamma(\nu) \tag{S7}$$

thus yields

$$\Gamma(\nu) = \frac{\mu^2\nu}{\varepsilon_0} \sum_{|\mathbf{p}|<\nu} \frac{1-|\hat{\mu}\cdot\mathbf{p}|^2/\nu^2}{\sqrt{1-p^2/\nu^2}} \sum_f \left| \langle f| \sum_{\mathbf{q}} e_{\mathbf{q}} h_{\mathbf{p}-\mathbf{q}} |i\rangle \right|^2 \delta(\omega_i - \omega_f - \nu). \tag{S8}$$

As the initial state, we consider the Chevy ansatz, described in the main text, with momentum $\mathbf{Q}$ and energy $E_{\mathrm{pol}}(\mathbf{Q})$:

$$|i\rangle = \Big(\alpha_{\mathbf{Q}} x^\dagger_{\mathbf{Q}} + \sum_{\substack{|\mathbf{q}|<k_F \\ |\mathbf{k}|>k_F}} \beta_{\mathbf{Q},\mathbf{k},\mathbf{q}} x^\dagger_{\mathbf{Q}+\mathbf{q}-\mathbf{k}} e'^\dagger_{\mathbf{k}} e'_{\mathbf{q}}\Big)|\mathrm{FS}\rangle. \tag{S9}$$

The simplest accessible final state is an empty Fermi sea, which gives rise to the first contribution to the decay rate,

$$\Gamma_1(\nu) = \frac{\mu^2\nu}{\varepsilon_0}|\alpha_{\mathbf{Q}}|^2 |\varphi_{\mathbf{Q}}(r=0)|^2 \frac{1-|\hat{\mu}\cdot\mathbf{Q}|^2/\nu^2}{\sqrt{1-|\mathbf{Q}|^2/\nu^2}} \Theta(\nu - |\mathbf{Q}|)\delta(E_{\mathrm{pol}}(\mathbf{Q})-\nu), \tag{S10}$$

where $\varphi_{\mathbf{Q}}(r=0) = \sum_{\mathbf{q}} \varphi_{\mathbf{Q}}(\mathbf{q})$ is the exciton wavefunction at vanishing separation between the electron and the hole. The dependence on the Fermi energy is implicit. This decay rate is nonzero only if the polaron is inside the light cone, $|\mathbf{Q}| < \nu$. It is therefore only relevant for states close to zero momentum but not the roton minimum. The expression further allows us to obtain the decay rate $\Gamma_0$ of an exciton at zero momentum and zero Fermi energy by setting $\mathbf{Q} = 0$ and $\alpha_{\mathbf{Q}} = 1$ and integrating over $\nu$. Hence,

$$\Gamma_0 = \frac{\mu^2\nu}{\varepsilon_0}|\varphi_0(r=0)|^2. \tag{S11}$$

Next, we consider final states in which an electron-hole pair is left behind in the $K$ valley but no in the $K'$ valley. This corresponds to the physical process denoted by $\Gamma_3$ in the main text. It is straightforward to show that

$$\Gamma_3(\nu) = \frac{\mu^2\nu}{\varepsilon_0}|\alpha_{\mathbf{Q}}|^2 \sum_{|\mathbf{p}|<\nu} \frac{1-|\hat{\mu}\cdot\mathbf{p}|^2/\nu^2}{\sqrt{1-p^2/\nu^2}} \sum_{|\mathbf{q}|<k_F} |\varphi_{\mathbf{Q}}(\mathbf{Q}+\mathbf{q}-\mathbf{p})|^2 \delta(\Omega_{\mathbf{Q}} - \varepsilon_{\mathbf{Q}+\mathbf{q}-\mathbf{p}} + \varepsilon_{\mathbf{q}} - \nu). \tag{S12}$$

The above expression can be simplified by noting that the in-plane photon momentum $\mathbf{p}$ is bounded by $\nu$, which is small compared to the relevent momentum scales of the TMD such as the Fermi momentum and the inverse Bohr radius. This allows us to set $\mathbf{p} = 0$ in the second sum such that the first sum can be evaluated directly,

$$\frac{1}{A}\sum_{|\mathbf{p}|<\nu} \frac{1-|\hat{\mu}\cdot\mathbf{p}|^2/\nu^2}{\sqrt{1-p^2/\nu^2}} = \frac{\nu^2}{3\pi}. \tag{S13}$$

yielding

$$\Gamma_3(\nu) \approx \frac{\mu^2\nu^3}{3\pi\varepsilon_0}|\alpha_{\mathbf{Q}}|^2 \sum_{|\mathbf{q}|<k_F} |\varphi_{\mathbf{Q}}(\mathbf{Q}+\mathbf{q})|^2 \delta(\Omega_{\mathbf{Q}} - \varepsilon_{\mathbf{Q}+\mathbf{q}} + \varepsilon_{\mathbf{q}} - \nu). \tag{S14}$$

A similar procedure can be applied to remaining two decay rates. For the process $\Gamma_2$, where an electron-hole pair remains in $K'$ but not in $K$, we obtain

$$\Gamma_2(\nu) \approx \frac{\mu^2\nu^3}{3\pi\varepsilon_0}|\varphi_0(r=0)|^2 \sum_{|\mathbf{q}|<k_F} |\beta_{\mathbf{Q},\mathbf{q},\mathbf{Q}+\mathbf{q}}|^2 \delta(\Omega_{\mathbf{Q}} - \varepsilon_{\mathbf{Q}+\mathbf{q}} + \varepsilon_{\mathbf{q}} - \nu), \tag{S15}$$

while for the process that leaves behind an excitation in each Fermi sea, the corresponding spectral decay rate is given by

$$\Gamma_4(\nu) \approx \frac{\mu^2\nu^3}{3\pi\varepsilon_0} \sum_{\substack{|\mathbf{q}|<k_F \\ |\mathbf{k}|,|\mathbf{k}'|>k_F}} |\beta_{\mathbf{Q},\mathbf{q},\mathbf{k}}|^2 |\varphi_{\mathbf{Q}-\mathbf{k}+\mathbf{q}}(\mathbf{k}')|^2 \Theta(k_F - |\mathbf{Q}-\mathbf{k}-\mathbf{k}'+\mathbf{q}|)\times$$
$$\delta(\Omega_{\mathbf{Q}} - \varepsilon_{\mathbf{k}} - \varepsilon_{\mathbf{k}'} + \varepsilon_{\mathbf{q}} + \varepsilon_{\mathbf{k}+\mathbf{k}'-\mathbf{q}-\mathbf{Q}} - \nu). \tag{S16}$$

* ocotlet@phys.ethz.ch
† wild@g.harvard.edu

[S1] T. C. Berkelbach, M. S. Hybertsen, and D. R. Reichman, Phys. Rev. B **88**, 045318 (2013).
[S2] A. Kormányos, G. Burkard, M. Gmitra, J. Fabian, V. Zólyomi, N. D. Drummond, and V. Fal'ko, 2D Mater. **2**, 022001 (2015).
[S3] H. Haug and S. W. Koch, *Quantum Theory of the Optical and Electronic Properties of Semiconductors*, 5th ed. (World Scientific, Singapore, 2009).
